# Supplementary material for: MR-WAVES: MR Water-diffusion And Vascular Effects Simulations
Source: arXiv:2503.01318 source file (2025-03-03)

# MR-WAVES: MR Water-diffusion And Vascular Effects Simulations

Thomas Coudert | Maitê Silva Martins Marçal | Aurélien Delphin | Antoine Barrier | Lila Cunge |  
Loïc Legris | Jan M Warnking | Benjamin Lemasson | Emmanuel L Barbier | Thomas Christen

## **SUPPLEMENTARY MATERIALS**

**FigureS1:** a) Parametric MRvF maps computed using a 20,000-entry zero-diffusion dictionary from the reference ( $Ref_{nodiff}$ ) and the proposed methods ( $MRWAVES_{nodiff}$ ). For this one animal, results are compared through a one-slice relative difference map and an all-slices relative difference histogram for each estimated parameter. b) Bland-Altman analyses across all animals of the study in the whole brain ROI.

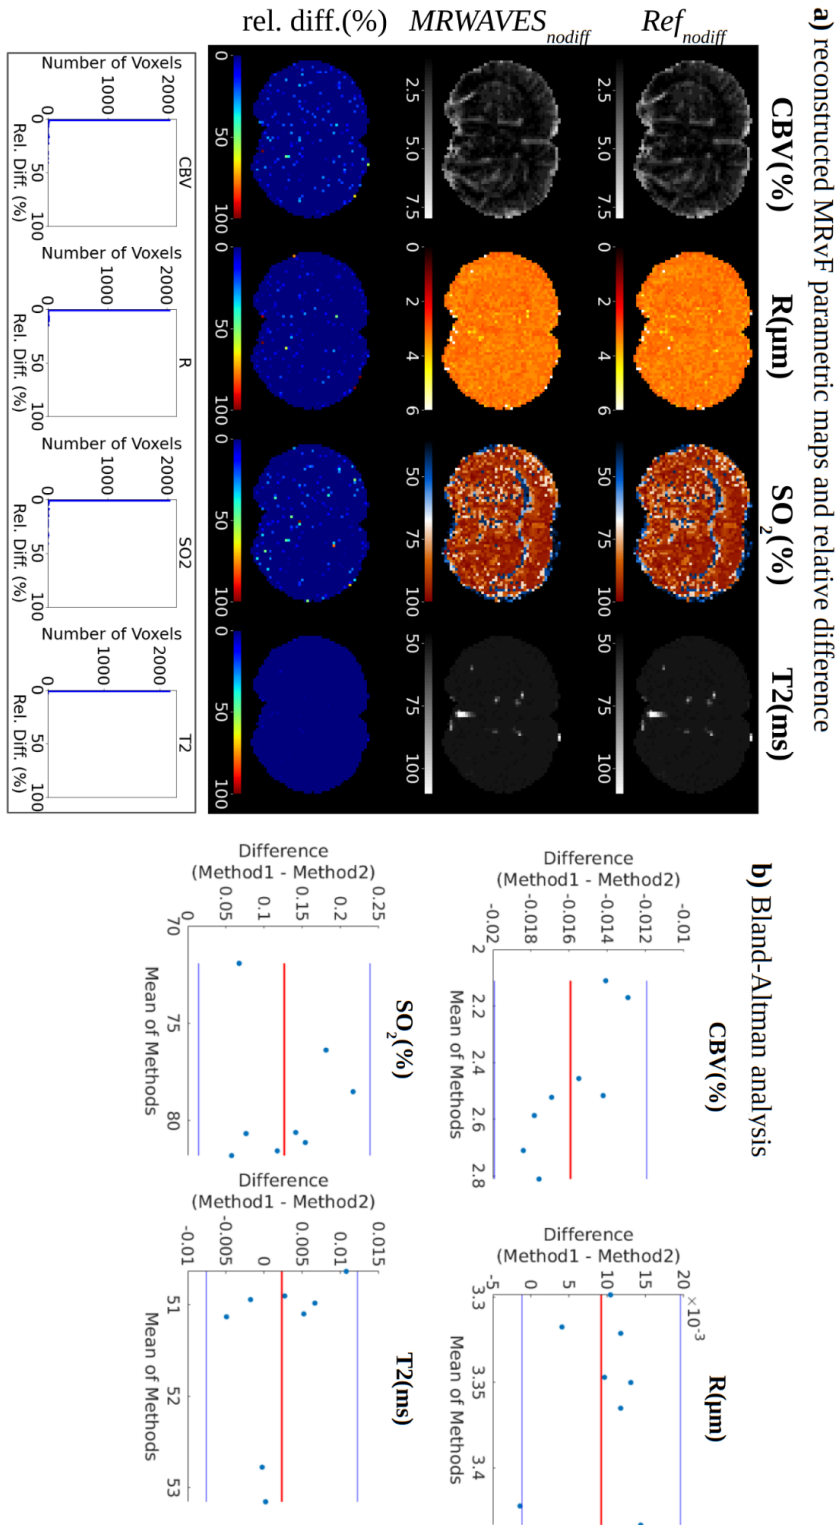

**FigureS2:** One slice example of MRvF parametric maps reconstructed from a 2000-entry dictionary computed with zero-diffusion using brute force method ( $Ref_{nodiff}$ , top), with an ADC of  $850\mu\text{m}^2/\text{s}$  using brute force method i.e. Gaussian kernel ( $Ref_{diff}$ , middle) and with an ADC of  $850\mu\text{m}^2/\text{s}$  using the proposed GRU-RNN ( $GRU_{diff}$ , bottom). Relative difference maps are also shown for each estimated parameter.

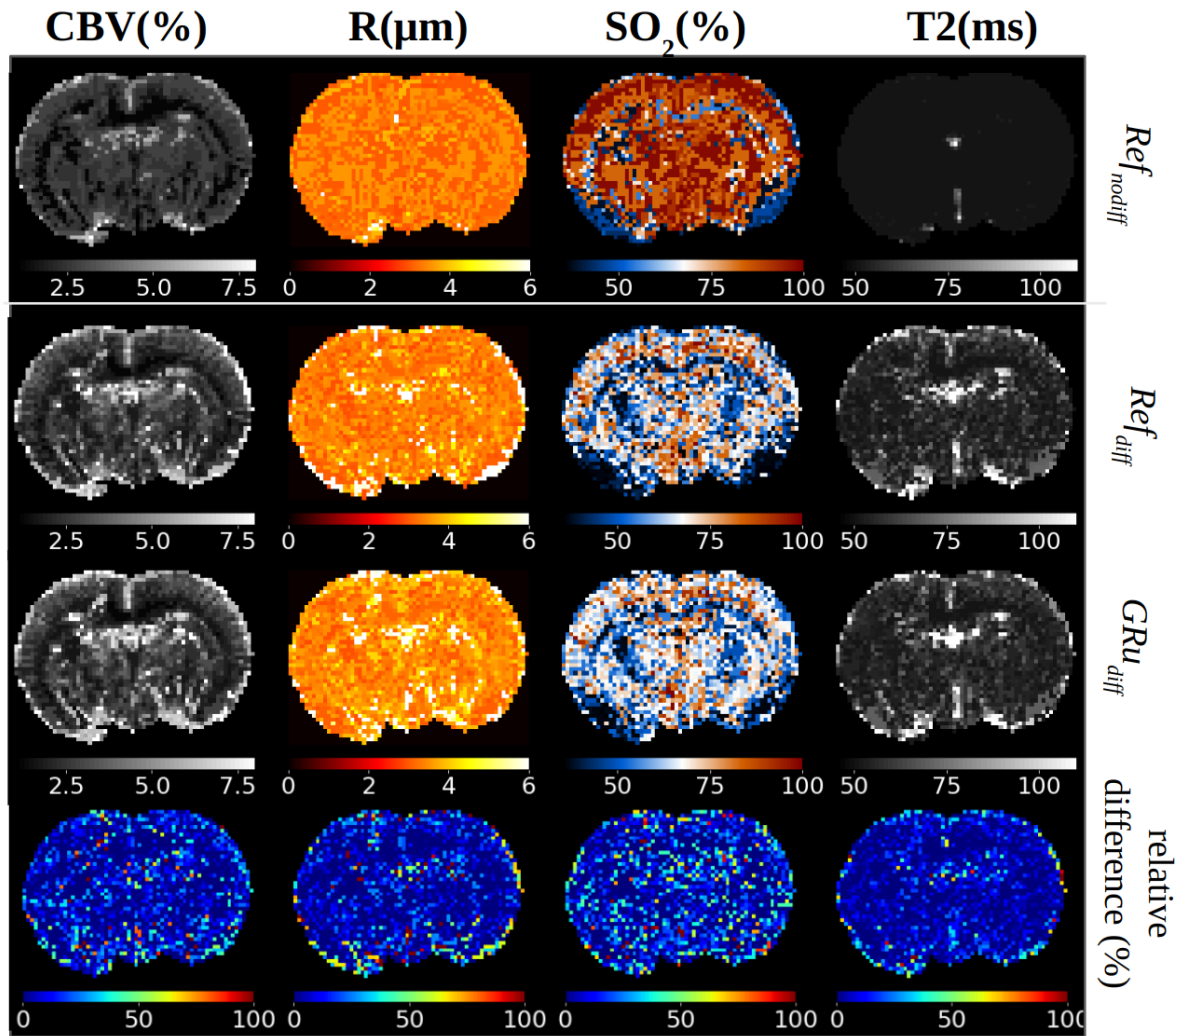

Supplement: Supplementary file 1 [file Supplementary_material_MRWAVES.pdf]
